# Supplementary material for: General supervised learning as change propagation with delta lenses
Source: arXiv:1911.12904 source file (2021-07-09)
Supplement: Supplementary file 1 [file accat-symLensAppendix.tex]

\section{Appendix. Algebra of bidirectional update propagation}
\newcommand\figr{\figref{fig:fbPpg-oper-laws}}

In Section \ref{sect-bx}, we considered operations of update propagation,
but did not specify any laws they must satisfy. Such laws are crucial for
capturing semantics, and the present section aims to specify algebraic laws
for BX. We will do it in an elementary way using tile algebra (rather than
categorically ---  it is non-trivial and left for a future work). We will begin
with the notion of an \emph{alignment \fwk} to formalize delta
composition ($*$ in Section \ref{sect-bx}), and then proceed to algebraic
structures modeling BX --- \emph{symmetric delta lenses}. (Note that the
lenses we will introduce here are different from those defined in
\cite{me-models11}.)

\begin{defin}%[adapted from \cite{me-models11}]
An \emph{\aln\ \fwk} is given by the following data.

(i) Two categories with pullbacks, \spaA\ and \spaB, called \emph{model
spaces}.  We will consider spans in these categories up to their
equivalence via a head isomorphism commuting with legs. That is, we will
work with equivalence classes of spans, and the term 'span' will refer to an
equivalence class of spans. Then span composition (via pullbacks) is
strictly associative, and we have categories (rather than bicategories) of
spans, $\mathsf{Span_1}(\spaA)$ and $\mathsf{Span_1}(\spaB)$. Their
subcategories consisting of spans with injective legs  will be denoted by
\spaspaA\ and \spaspaB\ resp.

Such spans are to be thought of as \emph{(model) updates}. They will be
depicted by vertical bi-directional arrows, for example, $a$ and $b$ in the
diagrams \figref{fig:align-oper}(a). We will assume that the upper node of
such an arrow is its formal source, and the lower one is the target; the
source is the the original (state of the) model, and the target is the
updated model. Thus, model evolution is directed down.

A span whose upper leg is identity (nothing deleted) is an \emph{insert
update}; it will be denoted by unidirectional arrows going down. Dually, a
span with identity lower leg is a \emph{delete update}; it will be denoted
by a unidirectional arrow going up (but the formal source of such an arrow
is still the upper node).

(ii) For any two objects, $A\in\spaA_0$ and $B\in\spaB_0$, there is a set
$R(A,B)$ of \emph{correspondences} (or \emph{corrs} in short) from
$A$ to $B$. Elements of $R(A, B)$ will be depicted by bi-directional
horizontal arrows, whose formal source is $A$ and the target is $B$.

Updates and corrs will also be called \emph{vertical \emph{and}
horizontal deltas}, resp.

(iii) Two diagram operations over corrs and updates called
\emph{forward} and \emph{backward} \emph{(re)\aln}. Their arities are
shown in \figref{fig:align-oper}(a) (output arrows are dashed). We will
also write $a*r$ for $\falt(a,r)$ and $r*b$ for $\balt(b,r)$. %Note that \aln\
%operations act on spans, \ie, arrows of \spaspaA\ and \spaspaB.
We will often skip the prefix 're' and say '\aln' to ease terminology.
\end{defin}

%
%{Note that computation of the initial corr \bilar{r}{A}{B} is beyond the
%re-alignment \fwk: the initial \aln\ (model matching) may need complex
%heuristic and other context dependent information. Hence, operations
%above are actually \emph{re-}alignment operations, but we will
%often call them alignments to ease terminology. %With this
%%reservation, below we will often call re-\aln\ operations simply
%%\emph{\aln}.
%}

%===beginFigure
\input{diag-alnFwk}
%===EndFigure

There are three laws regulating alignment. Identity updates do not
actually need realignment:
%\mylabelledformula{\idaltlaw}{
%\ide{}{A}*r = r = r*\ide{}{B}%
%}
$$
\ide{}{A}*r = r = r*\ide{}{B}%
\leqno (\idaltlaw)
$$
for any corr \bilar{r}{A}{B}.

The result of applying a sequence of interleaving forward and backward
alignments does not depend on the order of application as
shown in \figref{fig:align-oper}(b):%
%\mylabelledformula{(\altaltlaw)}{
%$(a*r)*b = a*(r*b)$%
%}
$$
(a*r)*b = a*(r*b) \leqno (\falt{-}\balt)
$$
for any corr $r$ and any updates $a,b$. %\in\spadela, r\in\spadelab, b\in\spadelb$.%
%\yxmodifyok{\footnote{We could also directly define \aln\ as arrow
%composition (with pre-involution if necessary); then \altaltlaw\ law is
%nothing but associativity.}}{\tr{\footnote{We could also directly define
%\aln\ as arrow composition (with pre-involution if necessary); then
%\altaltlaw\ law is nothing but associativity.}}}

We will call diagrams like those shown in \figref{fig:align-oper}(a,b)
\emph{commutative} if the arrow at the respective operation output is
indeed equal to that one computed by the operation. For example, diagram
(b) is commutative if $r'=a*r*b$.

Finally, alignment is compositional: for any consecutive updates
\flar{a}{A}{A'}, \flar{a'}{A'}{A''},  \flar{b}{B}{B'}, \flar{b'}{B'}{B''},
the following holds:
%as shown in
%\figref{fig:align-oper}(c) to be read as follows: if the two squares in the
%left diagram are \faln, the the outer rectangle is \faln\ as well.
$$%
a'*(a*r) = (a;a')*r \mbox{   and   }
(r*b)*b' = r*(b;b') \leqno (\altaltlaw)
$$
where $;$ denotes sequential span composition.
%Of course, these laws state nothing but associativity of composition.

It is easy to see that having an \aln\ \fwk\ amounts to having a functor
\flar{\alpha}{\spaspaA\times\spaspaB}{\setcat}.

\begin{defin}A \emph{symmetric delta lens} (briefly, an sd-lens) is a triple

\noindent $(\alpha,\fppg,\bppg)$ with
\flar{\alpha}{\spaspaA\times\spaspaB}{\setcat} an \aln\ \fwk, and \fppg,
\bppg\ two diagram operations over corrs and updates (called forward and
backward update propagation, resp.). The arities are specified in \figr(a)
with output arrows dashed and output nodes not framed. Sometimes we
will use a linear notation and write $b=a.\fppg(r)$ and $a=b.\bppg(r)$ for
the cases specified in the diagrams.
\end{defin}
{
\input{diag-sdLens-letters}
}%
Each operation must satisfy the following laws.

\textbf{\emph{Stability}} or \idppglaw\ law: if nothing changes on one
side, nothing happens on the other side as well, that is, identity mappings
are propagated into identity mappings as shown by diagrams \figr(b).

\textbf{\emph{Monotonicity}}: Insert updates are propagated into
inserts, and delete updates are propagated into deletes, as specified in
\figr(c).

\textbf{\emph{Monotonic Compositionality}} or \ppgppglaw\ law:
composition of two consecutive inserts is propagated into composition of
propagations as shown by the left diagram in \figref{fig:monot-PpgPpg}
(to be read as follows: if the two squares are \fppg, then the outer
rectangle is \fppg \ as well). The right diagram  specifies compositionality
for deletes. The same laws are formulated for \bppg.
\newarrow{Updto}----{>}
\newarrow{Derupdto}{}{dash}{}{dash}{>}

%-- version with letters A,B
\begin{wrapfigure}{R}{0.45\textwidth}
\vspace{-0.1cm}%
%\centering
\begin{tabular}{c@{\qquad}c} %@{\qquad}c@{\qquad}c}
%\multirow{2}{*}{%
    \begin{diagram}[w=\cellW,h=\cellH] %(a)
\dbox{A} & \rCorrto^r &\dbox{B}\\%
\dUpdto<a & \seTilearrow{\fppg}~~~
            & \dDerupdto>b \\%
\dbox{A'} & \rDercorrto^{r'} & B'  \\%
\dUpdto<{a'} & \seTilearrow{\fppg}~~~
            & \dDerupdto>b'\\%
            \dbox{A''} & \rDercorrto^{r''} & B''%
             &&\\
\end{diagram}%
% }%
  & %
%\multirow{2}{*}{%
    \begin{diagram}[w=\cellW,h=\cellH] %(a)
\dbox{A} & \rCorrto^r &\dbox{B}\\%
\uUpdto<a & \seTilearrow{\fppg}~~~
            & \uDerupdto>b \\%
\dbox{A'} & \rDercorrto^{r'} & B'  \\%
\uUpdto<{a'} & \seTilearrow{\fppg}~~~
            & \uDerupdto>b'\\%
            \dbox{A''} & \rDercorrto^{r''} & B''%
            &&\\
\end{diagram}%
% }%
\end{tabular}
\caption{Monotonic (\ppgppglaw) laws \label{fig:monot-PpgPpg}}%
\vspace{-0.1cm}
\end{wrapfigure}

Note that we do  not require compositionality for propagation of general
span updates. The point is that interleaving inserts and deletes can
annihilate, and lost information cannot be restored: see \cite{Foster07,
me-jot11,me-models11} for examples.

\textbf{\emph{Commutativity}}: Diagrams \figr(a) must be commutative
in the sense that $a*r*b = r'$.

Finally, forward and backward propagation must be coordinated with each
other by some \textbf{\emph{invertibility}} law. Given a corr
\flar{r}{A}{B}, an update \flar{a}{A}{A'} is propagated into update
$b=a.\fppg(r)$, which can be propagated back to update $a'=b.\bppg(r)$.
For an ideal situation of \emph{strong invertibility}, we should require
$a'=a$. Unfortunately, this does not hold in general because the
\spaspaA-specific part of the information is lost in passing from $a$ to
$b$, and cannot be restored \cite{me-models11}. However, it makes
sense to require the following  {\emph{weak invertibility}} specified in
\figref{fig:invert-laws}, which does hold in a majority of practically
interesting situations, \eg, for BX determined by TGG-rules
\cite{frank-models11}. The law \fbfppglaw\  says that although
$a_1=a.\fppg(r).\bppg(r)\neq a$, $a_1$ is equivalent to $a$ in the sense
that $a_1.\fppg(r) = a.\fppg(r)$. Similarly for the \bfbppglaw\ law.

\input{diag-weakInvert}

\bigskip
The notion of sd-lens is specified above in elementary terms using tile
algebra. Its categorical underpinning is not evident, and we only present
several brief remarks.

1) An \aln\ \fwk\  \flar{\alpha}{\spaspaA\times\spaspaB}{\setcat} can be
seen as a profunctor, if \spaA-arrows will be considered directed up (i.e.,
the formal source of update $a$ in diagram \figref{fig:align-oper}(a) is
$A'$, and the target is $A$). Then \aln\ amounts to a functor
\flar{\alpha}{{\spaspaA}^{\sf{op}}\times\spaspaB}{\setcat}, that is, a
profunctor \proflar{\alpha}{\spaspaB}{\spaspaA}. Note that reversing
arrows in \spaspaA\ actually changes the arity of operation \falt: now its
input is a pair $(a,r)$ with $a$ an update and $r$ a corr from the target of
$a$, and the output is a corr $r'$ from the source of $a$, that is, re\aln\
goes back in time.

2) Recall that operations \fppg\ and \bppg\ are functorial wrt. injective
arrows in \spaA, \spaB, not wrt. arrows in \spaspaA, \spaspaB. However, if
we try to resort to \spaA, \spaB\ entirely and define \aln\ wrt. arrows in
\spaA, \spaB, then we will need two \falt\ operations with different arities
for inserts and deletes, and two \balt\ operations with different arities for
inserts and deletes. We will then have four functors
\flar{\alpha_i}{\spaA\times\spaB}{\setcat} with $i$ ranging over
four-element set $\{insert, delete\}\times \{\spaA, \spaB\}$.

3)  The weak invertibility laws suggest that a Galois connection/adjunction
is somehow hidden in sd-lenses.

4) Working with chosen spans and pullbacks rather than with their
equivalence classes provides a more constructive setting (given we assume
the axiom of choice), but then associativity of span composition only holds
up to chosen natural isomorphisms, and  \spaspaA\ and \spaspaB\ have to
be considered bicategories rather than categories.

All in all, we hope that the categorical analysis of asymmetric delta lenses
developed by Johnson \etal\ \cite{joro10,joro12} could be extended to
capture the symmetric case too.

\endinput

\mysubsubsection{Basics (informally).}
 Diagrams \figr(a) specify the arities of two
diagram operations (the same as in \figref{fig:bx-scenario}(a) but with a
new visualization we will use in the Appendix). Horizontal arrows are
called \emph{correspondences} or just \emph{corrs}, or else
\emph{horizontal deltas}. Formally, they are assumed to be arrows going
from the left to the right. Vertical arrows denote \emph{updates}, and will
be also called \emph{vertical deltas} --- think of spans, whose legs are
injective. %Formally, vertical deltas are arrows going down.
An update span
whose upper leg is identity specifies the case with no deleted elements; we
will call such spans \emph{insert updates} and denote them by
unidirectional arrows going down. Dually, an update span with identity
lower leg is a \emph{delete update} denoted by unidirectional arrows
going up. Note that although update spans are denoted by bidirectional
arrows, the upper node is always the source, and the lower is the target
(so that the head of a delete update arrow point to its source rather than
the target!).

\mysubsubsection{Algebraic laws.} %: Stability and Monotonicity.}
A reasonable forward update propagation policy should satisfy the
following three basic requirements.

\emph{Invertibility.}  A basic requirement for \emph{bidirectional} model
\syncon\ is compatibility of propagation operations between themselves.

\mysubsubsection{Commutativity} The last requirement we need to
formulate is the condition that square diagrams resulted from update
propagation are to be commutative. To state such a condition, we need
operations of composing corrs with updates on the left and on the right.

\endinput
These and several other tile-shaped operations naturally appear in
algebraic modeling of BX-scenarios. Together they must satisfy a number
of equational laws, so that a coherent algebraic theory emerges.
Illustrating examples, and basics of tile algebra and its application to BX,
can be found in \cite{me-gttse-long}.  This theory provides a simple and
clear semantics for update propagation, which is really important for the
user of model sync tools.
