# Supplementary material for: General supervised learning as change propagation with delta lenses
Source: arXiv:1911.12904 source file (2021-07-09)
Supplement: Supplementary file 2 [file appendix.tex]

\section{Proof of the sequential lens composition associativity}

%We need to prove associativity of sequential composition and the presence of a monoidal structure (an associator and left- and right-unitors  satisfying required axioms). 

%\subsection{Associativity}
Let  
\frar{\ekk}{\spA}{\spB}, \frar{\ell}{\spB}{\spC}, \frar{\emm}{\spC}{\spD} be three consecutive lenses with parameter spaces \spP, \spQ, \spR\ resp. We will denote their components by an upper script, \eg, $\get^\ekk_p$ or $\putl^{\ell.\upd}_{q,B}$. % \ekk\ and $\ell$ as shown in \figkl, and \emm\ having the parameter space \spR.  
We need to prove $(\ekk;\ell);\emm=\ekk;(\ell;\emm)$. % for any three consecutive lenses 

We easily have associativity for the get part of the construction: $(\spP\timm\spQ)\timm\spR\cong\spP\timm(\spQ\timm\spR)$ (to be identified for equivalence classes), and $(\get^\ekk_p;\get^\ell_q);\get^\emm_r=\get^\ekk_p;(\get^\ell_q;\get^\emm_r)$.
%\clearpage
Associativity of puts is more involved. 
Suppose that we extended the diagram in \figkl\ with lens \emm\ data on the right, \ie, with a triangle prism, whose right face is a square $D_{pqr}D_{r'}D^@D'_r$ with diagonal \frar{\ome;\ome^@}{D_{pqr}}{D^@} where $r\in\spR$ is a parameter, $D_{pqr}=\get^\emm_r(C_{pq})$ and \frar{\ome}{D_{pqr}}{D'} is an arbitrary delta to be propagated to $\spP$ and \spA, and reflected as amendment $\ome^@=\putxyz{\emm.\self}{r}{C_{pq}}(\ome)$. 
We begin with term substitution in equations (\ref{eq:kldef1}-\ref{eq:kldef3}) in \conref{apa-seq}, which gives us equational definitions of all put operations: 
\begin{eqnarray}\label{eqna:kldef2}
	% row 6
		\frar{w.\putUL{\klbr.\upd}{pq,A} %
			&= &%
		((w.\putxy{q}{B_p}^{\ell.\req}).\putxy{p}{A}^{\ekk.\upd}}{p}{p'})
	\paar (w.\putl^{\ell.\upd}_{q,B_p}{:}~q\rightarrow q') \label{eq:eqna4}
	\\ % row 7
	\frar{w.\putl^{\klbr.\req}_{pq,A} %
		&=& %
		w.\putxy{q}{B_p}^{\ell.\req}.\putxy{p}{A}^{\ekk.\req}}{A}{A'}, \label{eq:eqna5}
	\\  % row 8
	% \mbox{ and }
	\frar{w.\putl^{\klbr.\self}_{pq,A} %
		&=& (w.\putl^{\ell.\self}_{q,B_p}) \,;\,
		(w.\putl^{\ell.\req}_{q,B_p}.%
		        \putl^{\ekk.\self}_{p,A}.\get^{\ell}_{q'})
	}{C'}{C^{@}}\rightarrow C^{@@} \label{eq:eqna6}
\end{eqnarray}
(note the interplay between different puts). Now we apply these definitions to the lens \klbr;\emm, \eg, for operation $\putl^{\klbr;\emm.\upd}$, and obtain the following inference (recall that pairs $(x,y)$ can also be denoted by $x\paar y$). 
\begin{eqnarray}   %\label{eqna:klm-proof}
\ome.\putl^{\klbr;\emm.\upd}_{(pq)r,A}
&=& % row 14
(\ome.\putl^{\emm.\req}_{r,C}.\putl^{\kl.\upd}_{pq,A}{:}~pq\rightarrow p'q')
\paarrx{(a)}
 (\ome.\putl^{\emm.\upd}_{r,C}{:}~r\rightarrow r')
\mbox{~~~~~by \eqref{eqna4}}
\\ &=& % row 15
\left((\ome.\putl^{\emm.\req}_{r,C}.\putl^{\ell.\req}_{q,B}).\putl^{\ekk.\upd}_{p,A} %
\right)\paar \left(
\ome.\putl^{\emm.\req}_{r,C}.\putl^{\ell.\upd}_{q,B}
\paar  \ldots\right)
%\ome.\putl^{\emm.\upd}_{r,C} 
\mbox{~~by \eqref{eqna4}\;\paar\ same}
\\ &=& % row 16
\ome.\putl^{\lmbr.\req}_{qr,B}.\putl^{\ekk.\upd}_{p,A}
\paarr 
\ome.\putl^{\lmbr.\upd}_{qr,B}
\mbox{~~~~by \eqref{eqna5} \paarr\ by \eqref{eqna4}}
\\ &=& % row 17
\ome.\putl^{\ekk;\lmbr.\upd}_{p(qr),A}
\mbox{~~~~by \eqref{eqna4}}
\end{eqnarray}
Associativity of $\putl^{(\ekk;\ell;\emm).\req}_{pqr,A}$ and $\putl^{(\ekk;\ell;\emm).\self}_{pqr,A}$ can be proved in a similar manner (using sequential associativity rather than monoidal associativity above).

\endinput 
\subsection{Monoidality}
In \citefst, Fong \etal\ prove that the category of codiscrete apa-lenses is sm by showing that the required monoidal structure is borrowed from Cartesian sm-category $(\setcat, \times)$. We can do the same with \catcat\ instead of \setcat. Indeed, any isomorphism between categories via a functor \frar{\iota}{\spA}{\spB} gives rise to a trivial apa-lens \frar{\ell(iota)}{\spA}{\spB} with the parameter space being \tcat, $\putl^\req$ being the inverse of $\iota$ and all $\putl^\self$ being identities. Then the monoidal structure in $(\catcat, \times)$ is adapted for \apalenscat.

\endinput

We also have %$w=\putxyz{\emm.\req}{}{}$
$w=\putxyz{\emm.\req}{r}{C_{pq}}(\ome)$ and 
$\frar{\eps=\putxyz{\emm.\upd}{r}{C_{pq}}(\ome)}{r}{r'}$. 
Then we extend the purple prism with the required fill-in arrows produced by functors $\get^\mu_r$ and $\get^\mu_{r'}$ as required.

, \eg, the full diagonal on the right face will be %$\ome;\ome^@;\get^\mu_{r'}(w^{\ekk;\ell.@})=
$\ome;\ome^@; $
